# Supplementary material for: Evaluation of imputation techniques with varying percentage of missing data
Source: arXiv:2109.04227 source file (2021-09-09)
Supplement: Supplementary file 1 [file Appendix.tex]

\begin{center}
	\begin{longtable}{ | c | c | c|}
		\caption{BoxPlot of RMSE Results}
		 \\ \hline	
		\hline\multicolumn{3}{|c|}
		{{ \tablename \ \thetable{} }}\\
		\hline{} & 	\frame{\includegraphics[width=0.33\textwidth, height=5mm]{Legends}}  &{} \\
		\hline
		\endhead
			
			\hline\multicolumn{3}{|r|}{{continued on next page}}\\
		\hline
		\endfoot
			
		\hline \multicolumn{3}{|r|}{{Continued on next page}} \\ \hline
		\endfoot
			
			 \hline
			\\
			\frame{\includegraphics[width=0.33\textwidth, height=50mm]{X0}}
			& 
			\frame{\includegraphics[width=0.33\textwidth, height=50mm]{X1}}
			& 
			\frame{\includegraphics[width=0.33\textwidth, height=50mm]{X2}}
				\\ \hline
			\\
			\frame{\includegraphics[width=0.33\textwidth, height=50mm]{X3}}
			& 
			\frame{\includegraphics[width=0.33\textwidth, height=50mm]{X4}}
			& 
			\frame{\includegraphics[width=0.33\textwidth, height=50mm]{X5}}
				\\ 
				\hline
			\\
			\frame{\includegraphics[width=0.33\textwidth, height=50mm]{X6}}
			& 
			\frame{\includegraphics[width=0.33\textwidth, height=50mm]{X8}}
			& 
			\frame{\includegraphics[width=0.33\textwidth, height=50mm]{X10}}
				\\ \hline
				\\
			\frame{\includegraphics[width=0.33\textwidth, height=50mm]{X11}}
			& 
			\frame{\includegraphics[width=0.33\textwidth, height=50mm]{X13}}
			& 
			\frame{\includegraphics[width=0.33\textwidth, height=50mm]{X14}}
			\\ \hline
			\\
			\frame{\includegraphics[width=0.33\textwidth, height=50mm]{X15}}
			& 
			\frame{\includegraphics[width=0.33\textwidth, height=50mm]{X16}}
			& 
			\frame{\includegraphics[width=0.33\textwidth, height=50mm]{X17}}
			\\ \hline
			\\
			\frame{\includegraphics[width=0.33\textwidth, height=50mm]{X18}}
			&
			\frame{\includegraphics[width=0.33\textwidth, height=50mm]{X19}}
			& 
			\frame{\includegraphics[width=0.33\textwidth, height=50mm]{X20}}
			\\ \hline
		\label{tbl:RMSEResults}
	\end{longtable}
\end{center}

%Source: https://tex.stackexchange.com/questions/201152/how-can-i-make-a-long-and-wide-table-fit-the-text-width

%ENTER THE VARIABLE IN AMELIA ROW
\begin{landscape}
	\begin{center}
		\small
		\setlength\tabcolsep{1pt}
		\begin{longtable}{c!{\hskip 0.1pt}>{\centering\arraybackslash}c!{\hskip 0.1pt}*{7}{|c}!{\hskip 0.1pt}*{7}{|c}!{\hskip 0.1pt}*{7}{|c}}
			\caption{Results based on RMSE}\\
			\toprule
			\multirow{2}{*}{Variable} & \multirow{2}{*}{\centering Algorithm}  & \multicolumn{7}{|c|}{5\% Missing} & \multicolumn{7}{|c|}{15\% Missing} & \multicolumn{7}{|c|}{25\% Missing}\\
			\cmidrule{3-23}
			&   &   $\mu$ & Median &  Q1  &  Q2  &  Q3 &  Q4  &  $\sigma$  & $\mu$ & Median &  Q1  &  Q2  &  Q3 &  Q4  &  $\sigma$  &$\mu$ & Median &  Q1  &  Q2  &  Q3 &  Q4  &  $\sigma$  \\
			\midrule\endhead
			\bottomrule\endfoot
			\multirow{6}[4]{*}{\textbf{X0}} & Mean  & 0.9972 & 0.9961 & 0.9735 & 0.9906 & 1.0047 & 1.0234 & 0.0115 & 0.9982 & 0.996 & 0.9863 & 0.9938 & 1.0015 & 1.0241 & 0.0073 & 1     & 1.0009 & 0.9831 & 0.995 & 1.0038 & 1.0136 & 0.0065 \\
			\cmidrule{2-23}          & MICE  & 1.1617 & 1.1626 & 1.113 & 1.1517 & 1.1725 & 1.2033 & 0.0156 & 1.1812 & 1.1814 & 1.1447 & 1.1749 & 1.1879 & 1.2071 & 0.01  & 1.2034 & 1.2043 & 1.1802 & 1.1976 & 1.2084 & 1.2245 & 0.0076 \\
			\cmidrule{2-23}          & Mi    & 1.414 & 1.4123 & 1.3757 & 1.4028 & 1.4265 & 1.4544 & 0.0176 & 1.4123 & 1.4123 & 1.3916 & 1.406 & 1.42  & 1.439 & 0.0099 & 1.4141 & 1.414 & 1.3988 & 1.4072 & 1.4197 & 1.4295 & 0.0076 \\
			\cmidrule{2-23}          & Amelia & 1.1784 & 1.178 & 1.1324 & 1.1675 & 1.1895 & 1.2285 & 0.0161 & 1.1941 & 1.1952 & 1.1563 & 1.1872 & 1.2009 & 1.2188 & 0.0103 & 1.211 & 1.211 & 1.1886 & 1.206 & 1.2158 & 1.2378 & 0.008 \\
			\cmidrule{2-23}          & Hmisc & 1.1639 & 1.1633 & 1.122 & 1.1541 & 1.1732 & 1.2151 & 0.0156 & 1.1835 & 1.1828 & 1.1611 & 1.1757 & 1.1902 & 1.2151 & 0.0101 & 1.2053 & 1.205 & 1.1865 & 1.2   & 1.211 & 1.2264 & 0.0077 \\
			\cmidrule{2-23}          & missForest & 0.7597 & 0.7542 & 0.7213 & 0.7464 & 0.7596 & 1.0013 & 0.0411 & 0.7858 & 0.7854 & 0.7684 & 0.7808 & 0.7901 & 0.8036 & 0.0077 & 0.8129 & 0.8131 & 0.7967 & 0.809 & 0.8162 & 0.9999 & 0.0135 \\
			\midrule
			\multirow{6}[4]{*}{\textbf{X1}} & Mean  & 0.9985 & 0.9976 & 0.8353 & 0.943 & 1.0455 & 1.2137 & 0.0788 & 0.9915 & 0.9894 & 0.8822 & 0.949 & 1.0407 & 1.1306 & 0.0573 & 1.0046 & 0.9977 & 0.8838 & 0.9696 & 1.0366 & 1.1061 & 0.0496 \\
			\cmidrule{2-23}          & MICE  & 0.5413 & 0.5342 & 0.4323 & 0.513 & 0.5665 & 0.7632 & 0.0455 & 0.587 & 0.585 & 0.506 & 0.5641 & 0.6089 & 0.7217 & 0.0322 & 0.6486 & 0.6471 & 0.5845 & 0.6297 & 0.6675 & 0.733 & 0.0277 \\
			\cmidrule{2-23}          & Mi    & 1.4107 & 1.4129 & 1.2638 & 1.3593 & 1.455 & 1.64  & 0.0706 & 1.3932 & 1.3904 & 1.3258 & 1.3648 & 1.4259 & 1.4943 & 0.0394 & 1.44  & 1.4469 & 1.3606 & 1.4059 & 1.4718 & 1.5292 & 0.0398 \\
			\cmidrule{2-23}          & Amelia & 0.5739 & 0.5676 & 0.5239 & 0.5539 & 0.5895 & 0.6778 & 0.0286 & 0.6165 & 0.6149 & 0.5762 & 0.6019 & 0.6308 & 0.674 & 0.0193 & 0.6745 & 0.674 & 0.6281 & 0.6607 & 0.6881 & 0.7263 & 0.0185 \\
			\cmidrule{2-23}          & Hmisc & 0.5389 & 0.534 & 0.4422 & 0.5086 & 0.5637 & 0.6717 & 0.042 & 0.5886 & 0.5852 & 0.5198 & 0.5644 & 0.6123 & 0.6815 & 0.0313 & 0.6535 & 0.6524 & 0.57  & 0.6293 & 0.6753 & 0.7468 & 0.0337 \\
			\cmidrule{2-23}          & missForest & 0.3596 & 0.3309 & 0.2594 & 0.3069 & 0.3569 & 1.1355 & 0.1364 & 0.4477 & 0.4027 & 0.3426 & 0.3741 & 0.433 & 1.106 & 0.1592 & 0.4722 & 0.4596 & 0.3996 & 0.4408 & 0.4834 & 0.9984 & 0.0791 \\
			\midrule
			\multirow{6}[12]{*}{\textbf{X2}} & Mean  & 0.9964 & 0.9954 & 0.8082 & 0.9509 & 1.0477 & 1.1756 & 0.0793 & 0.9979 & 0.9916 & 0.9255 & 0.9685 & 1.0263 & 1.1026 & 0.0409 & 0.9958 & 0.991 & 0.925 & 0.9722 & 1.0185 & 1.0876 & 0.04 \\
			\cmidrule{2-23}          & MICE  & 0.7471 & 0.7435 & 0.6594 & 0.7232 & 0.7703 & 0.8519 & 0.036 & 0.7769 & 0.7726 & 0.7208 & 0.7577 & 0.7932 & 0.8577 & 0.027 & 0.815 & 0.8161 & 0.7553 & 0.7984 & 0.8315 & 0.8743 & 0.0236 \\
			\cmidrule{2-23}          & Mi    & 1.4014 & 1.3986 & 1.2577 & 1.3487 & 1.4314 & 1.665 & 0.0745 & 1.399 & 1.3952 & 1.3359 & 1.3816 & 1.4139 & 1.4599 & 0.0271 & 1.3924 & 1.3873 & 1.3329 & 1.3711 & 1.4138 & 1.4673 & 0.0324 \\
			\cmidrule{2-23}          & Amelia & 0.7528 & 0.7503 & 0.6933 & 0.7352 & 0.7666 & 0.831 & 0.0232 & 0.778 & 0.7762 & 0.7318 & 0.7653 & 0.7888 & 0.8229 & 0.0184 & 0.8133 & 0.8121 & 0.7609 & 0.8   & 0.826 & 0.8608 & 0.0178 \\
			\cmidrule{2-23}          & Hmisc & 0.7505 & 0.75  & 0.6643 & 0.7245 & 0.7745 & 0.8685 & 0.0369 & 0.7779 & 0.7766 & 0.7118 & 0.7601 & 0.7937 & 0.8416 & 0.0261 & 0.8151 & 0.8158 & 0.75  & 0.7949 & 0.8324 & 0.9054 & 0.0256 \\
			\cmidrule{2-23}          & missForest & 0.5675 & 0.5455 & 0.4938 & 0.5249 & 0.5776 & 1.0808 & 0.0915 & 0.5775 & 0.5695 & 0.5307 & 0.554 & 0.5933 & 0.9715 & 0.043 & 0.6047 & 0.6   & 0.5621 & 0.5885 & 0.6217 & 0.652 & 0.022 \\
			\midrule
			\multirow{6}[12]{*}{\textbf{X3}} & Mean  & 1.0174 & 0.9971 & 0.8194 & 0.9295 & 1.0606 & 1.4417 & 0.1333 & 0.9864 & 0.9856 & 0.8627 & 0.9429 & 1.0243 & 1.1436 & 0.0676 & 0.9894 & 0.9912 & 0.8446 & 0.9556 & 1.0243 & 1.1043 & 0.0583 \\
			\cmidrule{2-23}          & MICE  & 0.4275 & 0.4224 & 0.3251 & 0.401 & 0.4539 & 0.5921 & 0.0428 & 0.494 & 0.4889 & 0.4362 & 0.4715 & 0.5111 & 0.6166 & 0.0316 & 0.5578 & 0.5553 & 0.4918 & 0.5423 & 0.5749 & 0.6257 & 0.0272 \\
			\cmidrule{2-23}          & Mi    & 1.431 & 1.406 & 1.3174 & 1.3537 & 1.473 & 1.8115 & 0.1011 & 1.4003 & 1.3998 & 1.3057 & 1.3674 & 1.4315 & 1.5146 & 0.0496 & 1.4073 & 1.4096 & 1.3047 & 1.3838 & 1.4308 & 1.491 & 0.0403 \\
			\cmidrule{2-23}          & Amelia & 0.5136 & 0.5123 & 0.4474 & 0.4967 & 0.5305 & 0.5803 & 0.0237 & 0.5714 & 0.5705 & 0.5211 & 0.5554 & 0.5867 & 0.6284 & 0.0218 & 0.6287 & 0.6271 & 0.5806 & 0.6173 & 0.6422 & 0.6718 & 0.0185 \\
			\cmidrule{2-23}          & Hmisc & 0.4579 & 0.4349 & 0.3299 & 0.4131 & 0.4674 & 1.0809 & 0.1042 & 0.507 & 0.5047 & 0.4367 & 0.4849 & 0.5262 & 0.6175 & 0.0324 & 0.5748 & 0.5717 & 0.517 & 0.5518 & 0.5914 & 0.6641 & 0.0309 \\
			\cmidrule{2-23}          & missForest & 0.3387 & 0.3142 & 0.2151 & 0.2847 & 0.3473 & 1.3226 & 0.1306 & 0.4099 & 0.372 & 0.3008 & 0.3503 & 0.3937 & 1.0732 & 0.147 & 0.4433 & 0.4347 & 0.3502 & 0.4133 & 0.4553 & 1.0945 & 0.0888 \\
			\midrule
			\multirow{6}[12]{*}{\textbf{X4}} & Mean  & 1.0067 & 1.0023 & 0.9467 & 0.9791 & 1.0302 & 1.1145 & 0.0365 & 0.9966 & 0.9954 & 0.9661 & 0.9838 & 1.009 & 1.038 & 0.0183 & 1.0006 & 0.9992 & 0.9715 & 0.9884 & 1.0084 & 1.0425 & 0.0158 \\
			\cmidrule{2-23}          & MICE  & 1.124 & 1.1193 & 1.0614 & 1.1021 & 1.1392 & 1.2487 & 0.0341 & 1.1323 & 1.1328 & 1.0807 & 1.1184 & 1.1438 & 1.2198 & 0.0206 & 1.1566 & 1.1567 & 1.1208 & 1.1455 & 1.1655 & 1.2146 & 0.0158 \\
			\cmidrule{2-23}          & Mi    & 1.4159 & 1.4106 & 1.3615 & 1.397 & 1.4335 & 1.5046 & 0.0274 & 1.4083 & 1.4059 & 1.3686 & 1.3972 & 1.4197 & 1.4429 & 0.0153 & 1.412 & 1.4119 & 1.3806 & 1.4032 & 1.4215 & 1.4416 & 0.0118 \\
			\cmidrule{2-23}          & Amelia & 1.1495 & 1.1464 & 1.0849 & 1.1297 & 1.165 & 1.2546 & 0.0285 & 1.1566 & 1.157 & 1.1194 & 1.1456 & 1.1681 & 1.1939 & 0.0162 & 1.1757 & 1.1747 & 1.1397 & 1.1653 & 1.1837 & 1.2269 & 0.0149 \\
			\cmidrule{2-23}          & Hmisc & 1.1232 & 1.1184 & 1.0516 & 1.1   & 1.1385 & 1.2479 & 0.035 & 1.1353 & 1.1346 & 1.0877 & 1.1204 & 1.1481 & 1.2172 & 0.0209 & 1.1584 & 1.1582 & 1.1164 & 1.1466 & 1.1686 & 1.2002 & 0.016 \\
			\cmidrule{2-23}          & missForest & 0.7635 & 0.7525 & 0.6931 & 0.7392 & 0.7784 & 1.0583 & 0.0499 & 0.7659 & 0.7623 & 0.7277 & 0.7526 & 0.7805 & 0.9975 & 0.0233 & 0.7969 & 0.7894 & 0.759 & 0.78  & 0.8018 & 1.0414 & 0.0401 \\
			\midrule
			\multirow{6}[12]{*}{\textbf{X5}} & Mean  & 1.0153 & 1.0158 & 0.8371 & 0.9286 & 1.0762 & 1.2897 & 0.1016 & 1.0078 & 1.006 & 0.9119 & 0.9721 & 1.0489 & 1.1225 & 0.0543 & 1.0062 & 1.0028 & 0.935 & 0.9865 & 1.0277 & 1.0856 & 0.0334 \\
			\cmidrule{2-23}          & MICE  & 0.4408 & 0.4382 & 0.3798 & 0.4206 & 0.4572 & 0.5284 & 0.0282 & 0.5038 & 0.501 & 0.4557 & 0.4865 & 0.5206 & 0.5765 & 0.0238 & 0.5628 & 0.5631 & 0.516 & 0.5479 & 0.576 & 0.6115 & 0.0196 \\
			\cmidrule{2-23}          & Mi    & 1.4287 & 1.4256 & 1.2555 & 1.3703 & 1.4735 & 1.641 & 0.0804 & 1.4247 & 1.423 & 1.3585 & 1.3937 & 1.4536 & 1.5155 & 0.0391 & 1.4182 & 1.4143 & 1.3627 & 1.4029 & 1.435 & 1.4712 & 0.0242 \\
			\cmidrule{2-23}          & Amelia & 0.4855 & 0.4829 & 0.4348 & 0.4713 & 0.4986 & 0.538 & 0.019 & 0.5424 & 0.5425 & 0.5041 & 0.5323 & 0.5525 & 0.5839 & 0.0165 & 0.5952 & 0.5962 & 0.5603 & 0.5849 & 0.6047 & 0.6342 & 0.0147 \\
			\cmidrule{2-23}          & Hmisc & 0.4569 & 0.4475 & 0.3725 & 0.432 & 0.469 & 0.6915 & 0.0495 & 0.5176 & 0.5116 & 0.4527 & 0.497 & 0.5312 & 0.6399 & 0.0312 & 0.573 & 0.572 & 0.5305 & 0.5605 & 0.5845 & 0.665 & 0.0209 \\
			\cmidrule{2-23}          & missForest & 0.3544 & 0.3395 & 0.2788 & 0.3229 & 0.3668 & 1.2193 & 0.095 & 0.4268 & 0.3946 & 0.3579 & 0.377 & 0.4191 & 1.1225 & 0.1311 & 0.4825 & 0.4479 & 0.4107 & 0.4324 & 0.464 & 1.0856 & 0.1379 \\
			\midrule
			\multirow{6}[12]{*}{\textbf{X6}} & Mean  & 0.9892 & 0.959 & 0.8195 & 0.9187 & 1.0532 & 1.2866 & 0.0975 & 1.0085 & 1.0012 & 0.9085 & 0.9697 & 1.0452 & 1.1764 & 0.0558 & 0.9854 & 0.9768 & 0.9021 & 0.9662 & 1.0148 & 1.0861 & 0.0391 \\
			\cmidrule{2-23}          & MICE  & 0.505 & 0.5012 & 0.4261 & 0.4806 & 0.5259 & 0.6347 & 0.0361 & 0.5584 & 0.5573 & 0.5013 & 0.5417 & 0.5755 & 0.6453 & 0.0259 & 0.605 & 0.6035 & 0.5517 & 0.591 & 0.6171 & 0.6716 & 0.021 \\
			\cmidrule{2-23}          & Mi    & 1.3959 & 1.3821 & 1.2748 & 1.3375 & 1.4403 & 1.6296 & 0.0745 & 1.3756 & 1.3725 & 1.2868 & 1.3456 & 1.4032 & 1.5098 & 0.0431 & 1.3927 & 1.3917 & 1.3311 & 1.3735 & 1.4128 & 1.4645 & 0.0282 \\
			\cmidrule{2-23}          & Amelia & 0.5083 & 0.5066 & 0.438 & 0.4919 & 0.5218 & 0.5932 & 0.0265 & 0.5655 & 0.565 & 0.5152 & 0.5521 & 0.5777 & 0.61  & 0.0187 & 0.6144 & 0.6117 & 0.5723 & 0.6033 & 0.6225 & 0.6612 & 0.0172 \\
			\cmidrule{2-23}          & Hmisc & 0.5197 & 0.5031 & 0.4312 & 0.4805 & 0.5352 & 0.7897 & 0.0692 & 0.5618 & 0.5582 & 0.4821 & 0.5436 & 0.5787 & 0.6839 & 0.0279 & 0.6088 & 0.6058 & 0.5577 & 0.5949 & 0.6241 & 0.6891 & 0.0216 \\
			\cmidrule{2-23}          & missForest & 0.4284 & 0.3932 & 0.3224 & 0.3746 & 0.4408 & 1.0874 & 0.1187 & 0.448 & 0.4394 & 0.3815 & 0.4266 & 0.4584 & 0.9878 & 0.0499 & 0.4847 & 0.4769 & 0.4327 & 0.4595 & 0.4942 & 1.0156 & 0.0597 \\
			\midrule
%			\multirow{6}[12]{*}{\textbf{X7}} & Mean  & 0.9928 & 0.9839 & 0.7673 & 0.9167 & 1.0594 & 1.187 & 0.0937 & 0.9998 & 0.9889 & 0.8818 & 0.9524 & 1.0398 & 1.1414 & 0.0634 & 1.0002 & 0.9934 & 0.8868 & 0.9606 & 1.0342 & 1.1326 & 0.0544 \\
%			\cmidrule{2-23}          & MICE  & 0.6641 & 0.66  & 0.5133 & 0.6152 & 0.7024 & 0.9439 & 0.0657 & 0.7131 & 0.7101 & 0.6127 & 0.6818 & 0.7427 & 0.8248 & 0.0433 & 0.7596 & 0.7567 & 0.6674 & 0.7366 & 0.785 & 0.8622 & 0.0357 \\
%			\cmidrule{2-23}          & Mi    & 1.4151 & 1.4132 & 1.2803 & 1.3655 & 1.4545 & 1.5587 & 0.0676 & 1.4304 & 1.4193 & 1.3437 & 1.4   & 1.4626 & 1.5212 & 0.0445 & 1.4188 & 1.4121 & 1.3292 & 1.3951 & 1.4495 & 1.5271 & 0.0444 \\
%			\cmidrule{2-23}          & Amelia & 0.7309 & 0.7322 & 0.6488 & 0.6992 & 0.7602 & 0.8242 & 0.0379 & 0.7708 & 0.7707 & 0.713 & 0.7519 & 0.7889 & 0.83  & 0.0266 & 0.8105 & 0.8096 & 0.7468 & 0.7937 & 0.8306 & 0.8886 & 0.0259 \\
%			\cmidrule{2-23}          & Hmisc & 0.6959 & 0.6923 & 0.5355 & 0.6402 & 0.7462 & 1.0265 & 0.0779 & 0.7469 & 0.745 & 0.6084 & 0.7184 & 0.7753 & 0.8831 & 0.0474 & 0.7873 & 0.7901 & 0.6574 & 0.7636 & 0.8093 & 0.9128 & 0.0389 \\
%			\cmidrule{2-23}          & missForest & 0.4284 & 0.4023 & 0.3286 & 0.3821 & 0.432 & 1.1307 & 0.1191 & 0.5043 & 0.4589 & 0.3742 & 0.4456 & 0.496 & 1.1414 & 0.1439 & 0.5184 & 0.5071 & 0.45  & 0.4928 & 0.5381 & 0.9972 & 0.0588 \\
%			\midrule
			\multirow{6}[12]{*}{\textbf{X8}} & Mean  & 0.9913 & 0.9868 & 0.8116 & 0.9169 & 1.0447 & 1.1847 & 0.093 & 0.9809 & 0.9725 & 0.8647 & 0.9232 & 1.0234 & 1.1813 & 0.0746 & 1.0013 & 0.9949 & 0.8995 & 0.96  & 1.0383 & 1.1874 & 0.0594 \\
			\cmidrule{2-23}          & MICE  & 0.4993 & 0.4954 & 0.4206 & 0.4757 & 0.5166 & 0.644 & 0.0334 & 0.558 & 0.5534 & 0.4898 & 0.5381 & 0.5757 & 0.6752 & 0.0314 & 0.6141 & 0.611 & 0.5435 & 0.5943 & 0.6326 & 0.7024 & 0.0291 \\
			\cmidrule{2-23}          & Mi    & 1.4089 & 1.4161 & 1.2495 & 1.3355 & 1.4684 & 1.5783 & 0.0882 & 1.3875 & 1.3776 & 1.3   & 1.3446 & 1.4163 & 1.5442 & 0.0544 & 1.4204 & 1.415 & 1.3423 & 1.3864 & 1.4521 & 1.5542 & 0.0441 \\
			\cmidrule{2-23}          & Amelia & 0.5177 & 0.5153 & 0.4657 & 0.5026 & 0.5301 & 0.5954 & 0.023 & 0.5793 & 0.5785 & 0.5266 & 0.5659 & 0.5939 & 0.6376 & 0.0218 & 0.6392 & 0.6385 & 0.587 & 0.6261 & 0.6535 & 0.7039 & 0.0225 \\
			\cmidrule{2-23}          & Hmisc & 0.5057 & 0.5025 & 0.4244 & 0.4797 & 0.5251 & 0.7181 & 0.0374 & 0.5652 & 0.5603 & 0.4831 & 0.5441 & 0.5794 & 0.6746 & 0.0343 & 0.6229 & 0.6175 & 0.5461 & 0.5989 & 0.6374 & 0.8167 & 0.0375 \\
			\cmidrule{2-23}          & missForest & 0.419 & 0.4016 & 0.3264 & 0.3803 & 0.4195 & 1.0568 & 0.1129 & 0.4498 & 0.4474 & 0.3711 & 0.4199 & 0.4725 & 0.5642 & 0.0396 & 0.499 & 0.4915 & 0.4433 & 0.4749 & 0.5164 & 0.9937 & 0.0453 \\
			\midrule
			\multirow{6}[12]{*}{\textbf{X9}} & Mean  & 0.9971 & 1.0018 & 0.9087 & 0.9717 & 1.0239 & 1.0865 & 0.0388 & 0.996 & 0.9962 & 0.9553 & 0.9833 & 1.011 & 1.0342 & 0.0196 & 0.9996 & 1.0003 & 0.9628 & 0.9879 & 1.0095 & 1.0471 & 0.0179 \\
			\cmidrule{2-23}          & MICE  & 0.9699 & 0.9693 & 0.886 & 0.9468 & 0.9886 & 1.0546 & 0.0302 & 1.01  & 1.0096 & 0.9492 & 0.9986 & 1.022 & 1.0557 & 0.0181 & 1.0474 & 1.048 & 1.0039 & 1.0372 & 1.0582 & 1.0926 & 0.0152 \\
			\cmidrule{2-23}          & Mi    & 1.4108 & 1.4121 & 1.2964 & 1.3766 & 1.4403 & 1.5301 & 0.0486 & 1.3989 & 1.4001 & 1.3568 & 1.3864 & 1.411 & 1.4402 & 0.0186 & 1.4059 & 1.4055 & 1.3662 & 1.3938 & 1.4194 & 1.4547 & 0.0182 \\
			\cmidrule{2-23}          & Amelia & 0.9805 & 0.98  & 0.9271 & 0.9679 & 0.9949 & 1.0534 & 0.0204 & 1.0183 & 1.0182 & 0.9815 & 1.0103 & 1.0266 & 1.0573 & 0.0136 & 1.0552 & 1.0552 & 1.0154 & 1.0465 & 1.0632 & 1.0856 & 0.0125 \\
			\cmidrule{2-23}          & Hmisc & 0.9721 & 0.9701 & 0.8866 & 0.953 & 0.9919 & 1.0675 & 0.0286 & 1.011 & 1.0104 & 0.95  & 0.9997 & 1.0237 & 1.0556 & 0.0174 & 1.0493 & 1.0497 & 1.0017 & 1.0375 & 1.061 & 1.0937 & 0.0165 \\
			\cmidrule{2-23}          & missForest & 0.6838 & 0.6815 & 0.6195 & 0.6638 & 0.6995 & 0.9794 & 0.0392 & 0.7159 & 0.7145 & 0.6832 & 0.7051 & 0.7213 & 1.0147 & 0.0274 & 0.7504 & 0.7455 & 0.7087 & 0.7336 & 0.7563 & 1.0229 & 0.0416 \\
			\midrule
			\multirow{6}[12]{*}{\textbf{X10}} & Mean  & 0.9935 & 0.9992 & 0.9036 & 0.9699 & 1.0213 & 1.0628 & 0.0395 & 1.0016 & 1.0016 & 0.9492 & 0.9865 & 1.0148 & 1.0598 & 0.0235 & 0.9938 & 0.9942 & 0.9539 & 0.981 & 1.0068 & 1.0366 & 0.0188 \\
			\cmidrule{2-23}          & MICE  & 0.6581 & 0.656 & 0.5934 & 0.6434 & 0.6737 & 0.7361 & 0.0224 & 0.6951 & 0.6949 & 0.6541 & 0.6871 & 0.7046 & 0.7288 & 0.0145 & 0.7338 & 0.7331 & 0.6999 & 0.7254 & 0.7421 & 0.7691 & 0.0128 \\
			\cmidrule{2-23}          & Mi    & 1.4102 & 1.4139 & 1.2939 & 1.3864 & 1.4345 & 1.5169 & 0.0403 & 1.408 & 1.4087 & 1.3678 & 1.396 & 1.4176 & 1.4512 & 0.0168 & 1.4079 & 1.4068 & 1.3786 & 1.3988 & 1.4171 & 1.4373 & 0.0131 \\
			\cmidrule{2-23}          & Amelia & 0.6804 & 0.6818 & 0.6321 & 0.6678 & 0.6904 & 0.7294 & 0.0165 & 0.7144 & 0.7146 & 0.6867 & 0.7068 & 0.7225 & 0.7417 & 0.0109 & 0.7483 & 0.7484 & 0.7221 & 0.7419 & 0.754 & 0.7808 & 0.0103 \\
			\cmidrule{2-23}          & Hmisc & 0.6612 & 0.6621 & 0.6017 & 0.6465 & 0.6745 & 0.7432 & 0.0225 & 0.698 & 0.6977 & 0.6524 & 0.6891 & 0.7078 & 0.7434 & 0.0147 & 0.7374 & 0.7358 & 0.7056 & 0.7279 & 0.7466 & 0.7792 & 0.0135 \\
			\cmidrule{2-23}          & missForest & 0.4572 & 0.445 & 0.4024 & 0.4333 & 0.4612 & 1.0017 & 0.0748 & 0.4934 & 0.4911 & 0.4597 & 0.4828 & 0.4992 & 0.9592 & 0.0326 & 0.5401 & 0.5267 & 0.4967 & 0.5168 & 0.535 & 1.0202 & 0.0832 \\
			\midrule
			\multirow{6}[12]{*}{\textbf{X11}} & Mean  & 1.0012 & 0.9995 & 0.9414 & 0.9841 & 1.0208 & 1.0571 & 0.0252 & 1.0018 & 1.0004 & 0.9696 & 0.9931 & 1.0106 & 1.042 & 0.0134 & 1.0011 & 0.9999 & 0.9784 & 0.9886 & 1.0099 & 1.0381 & 0.0145 \\
			\cmidrule{2-23}          & MICE  & 0.4052 & 0.4017 & 0.3559 & 0.3901 & 0.4194 & 0.4698 & 0.0216 & 0.5699 & 0.5689 & 0.5296 & 0.5615 & 0.5791 & 0.6146 & 0.0139 & 0.6776 & 0.677 & 0.6413 & 0.6694 & 0.6859 & 0.7206 & 0.0122 \\
			\cmidrule{2-23}          & Mi    & 1.4172 & 1.4168 & 1.3442 & 1.3944 & 1.4413 & 1.4939 & 0.0299 & 1.4298 & 1.4282 & 1.3978 & 1.4234 & 1.4397 & 1.463 & 0.0126 & 1.4145 & 1.4132 & 1.3838 & 1.4054 & 1.4249 & 1.4458 & 0.0142 \\
			\cmidrule{2-23}          & Amelia & 0.3872 & 0.3864 & 0.3474 & 0.3779 & 0.3972 & 0.438 & 0.0151 & 0.534 & 0.5342 & 0.4982 & 0.5284 & 0.5391 & 0.5594 & 0.0096 & 0.6441 & 0.6441 & 0.6209 & 0.6365 & 0.6499 & 0.688 & 0.0104 \\
			\cmidrule{2-23}          & Hmisc & 0.3997 & 0.3981 & 0.3649 & 0.3868 & 0.4118 & 0.4493 & 0.0173 & 0.5602 & 0.5594 & 0.525 & 0.5503 & 0.5699 & 0.6033 & 0.0151 & 0.6671 & 0.6672 & 0.636 & 0.6564 & 0.6791 & 0.6993 & 0.0142 \\
			\cmidrule{2-23}          & missForest & 0.2979 & 0.2847 & 0.2516 & 0.2728 & 0.2981 & 1.018 & 0.0924 & 0.4012 & 0.386 & 0.3555 & 0.3805 & 0.3938 & 1.0169 & 0.094 & 0.469 & 0.4569 & 0.4357 & 0.4506 & 0.4631 & 1.0261 & 0.0777 \\
			\midrule
			\multirow{6}[12]{*}{\textbf{X12}} & Mean  & 1.0022 & 1.0001 & 0.9252 & 0.9691 & 1.0249 & 1.1141 & 0.0403 & 1.0006 & 1.0033 & 0.9375 & 0.9796 & 1.0244 & 1.0643 & 0.0309 & 0.9957 & 0.995 & 0.9601 & 0.9762 & 1.0136 & 1.0544 & 0.022 \\
			\cmidrule{2-23}          & MICE  & 1.3083 & 1.3056 & 1.1982 & 1.2775 & 1.3395 & 1.4271 & 0.0448 & 1.3161 & 1.3168 & 1.2297 & 1.2967 & 1.3358 & 1.3823 & 0.0284 & 1.3201 & 1.3208 & 1.26  & 1.3054 & 1.335 & 1.3807 & 0.0226 \\
			\cmidrule{2-23}          & Mi    & 1.4218 & 1.4102 & 1.2939 & 1.3844 & 1.4789 & 1.5636 & 0.0601 & 1.4389 & 1.4416 & 1.3828 & 1.4238 & 1.4564 & 1.486 & 0.0224 & 1.4104 & 1.4084 & 1.3634 & 1.3959 & 1.4252 & 1.4686 & 0.0229 \\
			\cmidrule{2-23}          & Amelia & 1.3109 & 1.3077 & 1.227 & 1.2891 & 1.3301 & 1.4122 & 0.0335 & 1.3179 & 1.3191 & 1.2477 & 1.3019 & 1.3336 & 1.3843 & 0.0229 & 1.3227 & 1.3232 & 1.287 & 1.3092 & 1.3335 & 1.3719 & 0.0179 \\
			\cmidrule{2-23}          & Hmisc & 1.3046 & 1.2969 & 1.1825 & 1.2722 & 1.3308 & 1.4349 & 0.0447 & 1.3139 & 1.3134 & 1.2275 & 1.2951 & 1.3324 & 1.3841 & 0.0275 & 1.3189 & 1.3182 & 1.2637 & 1.3057 & 1.3317 & 1.3705 & 0.0205 \\
			\cmidrule{2-23}          & missForest & 0.9173 & 0.9112 & 0.8504 & 0.8895 & 0.9394 & 1.0446 & 0.0377 & 0.9276 & 0.9307 & 0.8622 & 0.9062 & 0.9488 & 0.9889 & 0.0287 & 0.9346 & 0.9331 & 0.8948 & 0.9187 & 0.9482 & 0.9959 & 0.0203 \\
			\midrule
			\multirow{6}[12]{*}{\textbf{X13}} & Mean  & 1.0047 & 1.0039 & 0.9784 & 0.9968 & 1.0126 & 1.0334 & 0.0131 & 0.9995 & 0.9991 & 0.9838 & 0.9937 & 1.0051 & 1.0239 & 0.0089 & 1.0006 & 1.0007 & 0.9858 & 0.9947 & 1.0063 & 1.019 & 0.0084 \\
			\cmidrule{2-23}          & MICE  & 1.1408 & 1.1412 & 1.0622 & 1.1264 & 1.158 & 1.1948 & 0.0235 & 1.153 & 1.1531 & 1.1222 & 1.1442 & 1.1619 & 1.1835 & 0.0119 & 1.1682 & 1.168 & 1.1385 & 1.1621 & 1.1747 & 1.2005 & 0.0097 \\
			\cmidrule{2-23}          & Mi    & 1.4127 & 1.4124 & 1.3569 & 1.3959 & 1.4355 & 1.4727 & 0.0245 & 1.4034 & 1.4027 & 1.3813 & 1.3979 & 1.4086 & 1.4266 & 0.0098 & 1.4085 & 1.4081 & 1.3881 & 1.4029 & 1.4153 & 1.4285 & 0.0085 \\
			\cmidrule{2-23}          & Amelia & 1.1631 & 1.1628 & 1.1176 & 1.1509 & 1.1759 & 1.2096 & 0.018 & 1.1726 & 1.1719 & 1.1428 & 1.1673 & 1.1787 & 1.1976 & 0.01  & 1.1879 & 1.1874 & 1.1598 & 1.1815 & 1.1942 & 1.2187 & 0.0094 \\
			\cmidrule{2-23}          & Hmisc & 1.1412 & 1.1418 & 1.0803 & 1.1247 & 1.1561 & 1.217 & 0.0224 & 1.1541 & 1.1547 & 1.1182 & 1.1472 & 1.1621 & 1.1937 & 0.012 & 1.1712 & 1.1711 & 1.1378 & 1.1634 & 1.1777 & 1.2018 & 0.0107 \\
			\cmidrule{2-23}          & missForest & 0.7578 & 0.7548 & 0.717 & 0.7423 & 0.7654 & 1.0181 & 0.0357 & 0.7725 & 0.7729 & 0.7474 & 0.7667 & 0.778 & 0.7989 & 0.0093 & 0.7933 & 0.7928 & 0.7785 & 0.7864 & 0.7973 & 1.0118 & 0.0159 \\
			\midrule
			\multirow{6}[12]{*}{\textbf{X14}} & Mean  & 1.0058 & 1.0037 & 0.9618 & 0.9883 & 1.0208 & 1.0886 & 0.0257 & 0.9976 & 0.9996 & 0.9607 & 0.9875 & 1.0071 & 1.0334 & 0.0159 & 0.9993 & 0.9974 & 0.9789 & 0.9903 & 1.0093 & 1.0262 & 0.0123 \\
			\cmidrule{2-23}          & MICE  & 0.4067 & 0.4045 & 0.3611 & 0.392 & 0.4195 & 0.4722 & 0.0207 & 0.5662 & 0.5672 & 0.5331 & 0.5564 & 0.5739 & 0.6082 & 0.0134 & 0.6758 & 0.6754 & 0.6365 & 0.6674 & 0.6836 & 0.7087 & 0.0125 \\
			\cmidrule{2-23}          & Mi    & 1.4144 & 1.4177 & 1.328 & 1.3981 & 1.4317 & 1.4838 & 0.0287 & 1.4112 & 1.4109 & 1.3826 & 1.4011 & 1.4195 & 1.4455 & 0.014 & 1.416 & 1.4163 & 1.3892 & 1.4074 & 1.4246 & 1.4376 & 0.0113 \\
			\cmidrule{2-23}          & Amelia & 0.3863 & 0.385 & 0.3492 & 0.3758 & 0.3965 & 0.4286 & 0.0151 & 0.5298 & 0.5293 & 0.4975 & 0.5242 & 0.5356 & 0.5622 & 0.0098 & 0.6422 & 0.6421 & 0.611 & 0.6351 & 0.6485 & 0.6819 & 0.0106 \\
			\cmidrule{2-23}          & Hmisc & 0.4052 & 0.4007 & 0.3591 & 0.3898 & 0.4138 & 0.5268 & 0.026 & 0.5575 & 0.5563 & 0.5185 & 0.5479 & 0.5666 & 0.6064 & 0.0147 & 0.665 & 0.6664 & 0.633 & 0.6554 & 0.6752 & 0.6947 & 0.0139 \\
			\cmidrule{2-23}          & missForest & 0.3118 & 0.2903 & 0.2615 & 0.2783 & 0.3004 & 1.0208 & 0.1191 & 0.3886 & 0.3843 & 0.3489 & 0.3786 & 0.3933 & 0.9986 & 0.0411 & 0.4603 & 0.4591 & 0.4359 & 0.4539 & 0.4675 & 0.4879 & 0.0095 \\
			\midrule
			\multirow{6}[12]{*}{\textbf{X15}} & Mean  & 0.9979 & 0.9978 & 0.9238 & 0.9772 & 1.0218 & 1.107 & 0.0343 & 0.9999 & 1.0017 & 0.9588 & 0.9857 & 1.0129 & 1.0436 & 0.019 & 0.9946 & 0.9942 & 0.9648 & 0.9803 & 1.0016 & 1.0308 & 0.0166 \\
			\cmidrule{2-23}          & MICE  & 1.1375 & 1.1349 & 1.0275 & 1.1174 & 1.156 & 1.2488 & 0.033 & 1.1641 & 1.1624 & 1.0974 & 1.1492 & 1.1767 & 1.2689 & 0.0232 & 1.1815 & 1.1803 & 1.1386 & 1.1707 & 1.1916 & 1.2401 & 0.0158 \\
			\cmidrule{2-23}          & Mi    & 1.4055 & 1.4043 & 1.3098 & 1.3745 & 1.4382 & 1.4835 & 0.0403 & 1.4115 & 1.4126 & 1.375 & 1.3995 & 1.4236 & 1.4537 & 0.0166 & 1.419 & 1.4192 & 1.3807 & 1.4039 & 1.4305 & 1.467 & 0.0183 \\
			\cmidrule{2-23}          & Amelia & 1.1481 & 1.1457 & 1.0823 & 1.13  & 1.1658 & 1.2421 & 0.0264 & 1.1668 & 1.1677 & 1.1224 & 1.1564 & 1.1765 & 1.2169 & 0.0158 & 1.1835 & 1.1831 & 1.146 & 1.174 & 1.1926 & 1.229 & 0.0143 \\
			\cmidrule{2-23}          & Hmisc & 1.1374 & 1.1331 & 1.0413 & 1.1113 & 1.1582 & 1.2983 & 0.037 & 1.1634 & 1.1624 & 1.1177 & 1.1505 & 1.1771 & 1.2178 & 0.02  & 1.1811 & 1.1797 & 1.1364 & 1.1695 & 1.1916 & 1.2316 & 0.0167 \\
			\cmidrule{2-23}          & missForest & 0.7759 & 0.7646 & 0.7078 & 0.7422 & 0.7934 & 1.0241 & 0.0559 & 0.797 & 0.7942 & 0.759 & 0.7864 & 0.8052 & 0.9906 & 0.0221 & 0.8145 & 0.8118 & 0.7839 & 0.8042 & 0.8238 & 0.8562 & 0.0149 \\
			\midrule
			\multirow{6}[12]{*}{\textbf{X16}} & Mean  & 1.0144 & 0.9966 & 0.9162 & 0.9817 & 1.0236 & 1.6872 & 0.102 & 1.0121 & 1.0009 & 0.9482 & 0.9875 & 1.0119 & 1.3032 & 0.0618 & 0.9946 & 0.9953 & 0.9227 & 0.9855 & 1.0094 & 1.0483 & 0.0246 \\
			\cmidrule{2-23}          & MICE  & 1.1489 & 1.1312 & 1.0378 & 1.1093 & 1.1534 & 1.8268 & 0.1045 & 1.1591 & 1.149 & 1.0765 & 1.1335 & 1.1604 & 1.4828 & 0.0568 & 1.1669 & 1.168 & 1.0833 & 1.1565 & 1.1789 & 1.2753 & 0.0267 \\
			\cmidrule{2-23}          & Mi    & 1.4224 & 1.4127 & 1.336 & 1.3818 & 1.4314 & 2.0013 & 0.0912 & 1.4183 & 1.4086 & 1.3634 & 1.4006 & 1.4226 & 1.6385 & 0.0466 & 1.4031 & 1.4016 & 1.3613 & 1.3921 & 1.4178 & 1.4415 & 0.0186 \\
			\cmidrule{2-23}          & Amelia & 1.1542 & 1.1408 & 1.0561 & 1.1251 & 1.1548 & 1.7686 & 0.0896 & 1.1674 & 1.1549 & 1.1128 & 1.1461 & 1.1685 & 1.4107 & 0.0515 & 1.1725 & 1.1727 & 1.0877 & 1.1643 & 1.1831 & 1.222 & 0.0192 \\
			\cmidrule{2-23}          & Hmisc & 1.145 & 1.1306 & 1.0227 & 1.1131 & 1.1512 & 1.7348 & 0.0929 & 1.1586 & 1.149 & 1.0737 & 1.1343 & 1.1664 & 1.4089 & 0.0523 & 1.1649 & 1.1672 & 1.0652 & 1.1539 & 1.1772 & 1.2523 & 0.0251 \\
			\cmidrule{2-23}          & missForest & 0.7819 & 0.7532 & 0.7051 & 0.7397 & 0.7783 & 1.5344 & 0.1201 & 0.7993 & 0.7822 & 0.7351 & 0.7731 & 0.7991 & 1.1224 & 0.0694 & 0.8012 & 0.8028 & 0.7448 & 0.7923 & 0.8125 & 0.8544 & 0.0202 \\
			\midrule
			\multirow{6}[12]{*}{\textbf{X17}} & Mean  & 1     & 1.0037 & 0.9592 & 0.986 & 1.0179 & 1.0418 & 0.0218 & 0.9972 & 0.995 & 0.9671 & 0.9886 & 1.005 & 1.0294 & 0.0124 & 0.9977 & 0.9961 & 0.9696 & 0.9886 & 1.0058 & 1.0237 & 0.0121 \\
			\cmidrule{2-23}          & MICE  & 0.8675 & 0.8683 & 0.8232 & 0.8572 & 0.8789 & 0.9197 & 0.0169 & 0.9038 & 0.9028 & 0.8771 & 0.8955 & 0.9118 & 0.9309 & 0.0113 & 0.9445 & 0.9449 & 0.914 & 0.9375 & 0.9507 & 0.9711 & 0.0102 \\
			\cmidrule{2-23}          & Mi    & 1.411 & 1.4147 & 1.3578 & 1.3943 & 1.4294 & 1.4729 & 0.0242 & 1.4252 & 1.4247 & 1.3926 & 1.418 & 1.4334 & 1.4516 & 0.0114 & 1.4091 & 1.4078 & 1.3754 & 1.3995 & 1.4178 & 1.4423 & 0.0132 \\
			\cmidrule{2-23}          & Amelia & 0.8679 & 0.8683 & 0.8253 & 0.855 & 0.8815 & 0.9094 & 0.0163 & 0.9032 & 0.9025 & 0.8827 & 0.8967 & 0.9091 & 0.932 & 0.0094 & 0.9428 & 0.9422 & 0.9165 & 0.935 & 0.9481 & 0.985 & 0.0111 \\
			\cmidrule{2-23}          & Hmisc & 0.8683 & 0.8688 & 0.8181 & 0.857 & 0.8801 & 0.9266 & 0.0176 & 0.9049 & 0.9039 & 0.878 & 0.8954 & 0.913 & 0.9403 & 0.0122 & 0.9465 & 0.9461 & 0.916 & 0.9408 & 0.9524 & 0.9782 & 0.0105 \\
			\cmidrule{2-23}          & missForest & 0.6102 & 0.6055 & 0.5682 & 0.5888 & 0.6142 & 1.0133 & 0.0554 & 0.6342 & 0.6342 & 0.6187 & 0.6269 & 0.641 & 0.6548 & 0.0091 & 0.6668 & 0.6668 & 0.6406 & 0.6596 & 0.6725 & 0.6923 & 0.0099 \\
			\midrule
			\multirow{6}[12]{*}{\textbf{X18}} & Mean  & 1.0026 & 0.9965 & 0.958 & 0.9829 & 1.0192 & 1.0682 & 0.0254 & 0.9976 & 0.9987 & 0.9713 & 0.9872 & 1.0074 & 1.0218 & 0.0133 & 1.0016 & 1.0011 & 0.9873 & 0.994 & 1.0074 & 1.0292 & 0.0094 \\
			\cmidrule{2-23}          & MICE  & 0.8377 & 0.8371 & 0.7907 & 0.824 & 0.8506 & 0.8917 & 0.0211 & 0.8752 & 0.875 & 0.8464 & 0.8674 & 0.8833 & 0.9044 & 0.0119 & 0.9214 & 0.9209 & 0.8945 & 0.9153 & 0.9277 & 0.9456 & 0.0096 \\
			\cmidrule{2-23}          & Mi    & 1.4165 & 1.4182 & 1.3732 & 1.3967 & 1.4323 & 1.474 & 0.0235 & 1.413 & 1.4127 & 1.3817 & 1.4049 & 1.4225 & 1.4425 & 0.0124 & 1.4134 & 1.4123 & 1.3902 & 1.4086 & 1.4196 & 1.4392 & 0.0103 \\
			\cmidrule{2-23}          & Amelia & 0.8387 & 0.8395 & 0.7924 & 0.8263 & 0.8503 & 0.8971 & 0.0175 & 0.8765 & 0.8761 & 0.8499 & 0.8704 & 0.8834 & 0.905 & 0.0099 & 0.9217 & 0.921 & 0.9005 & 0.9154 & 0.9275 & 0.9489 & 0.0088 \\
			\cmidrule{2-23}          & Hmisc & 0.8403 & 0.84  & 0.7863 & 0.8258 & 0.8554 & 0.9028 & 0.0217 & 0.877 & 0.8768 & 0.8443 & 0.8686 & 0.8849 & 0.9068 & 0.0119 & 0.9226 & 0.9224 & 0.8953 & 0.9156 & 0.9291 & 0.9514 & 0.0094 \\
			\cmidrule{2-23}          & missForest & 0.6033 & 0.5915 & 0.5497 & 0.5766 & 0.6073 & 1.0047 & 0.0683 & 0.6442 & 0.6235 & 0.5987 & 0.6153 & 0.631 & 1.0138 & 0.0861 & 0.6657 & 0.6585 & 0.6404 & 0.6539 & 0.6643 & 1.0084 & 0.0488 \\
			\midrule
			\multirow{6}[12]{*}{\textbf{X19}} & Mean  & 1.0015 & 1.0012 & 0.961 & 0.9881 & 1.0086 & 1.046 & 0.0185 & 0.9997 & 0.9992 & 0.9743 & 0.9922 & 1.0078 & 1.0263 & 0.0113 & 1.0017 & 1.0013 & 0.9878 & 0.997 & 1.0055 & 1.0209 & 0.0082 \\
			\cmidrule{2-23}          & MICE  & 1.3533 & 1.353 & 1.2819 & 1.3368 & 1.3696 & 1.4101 & 0.0237 & 1.3558 & 1.356 & 1.3193 & 1.3461 & 1.3661 & 1.3929 & 0.0137 & 1.3612 & 1.3614 & 1.337 & 1.3546 & 1.3678 & 1.3912 & 0.0109 \\
			\cmidrule{2-23}          & Mi    & 1.4142 & 1.4132 & 1.3448 & 1.3988 & 1.4304 & 1.4795 & 0.0253 & 1.4142 & 1.4129 & 1.3839 & 1.4069 & 1.4236 & 1.4432 & 0.0129 & 1.4121 & 1.4102 & 1.3911 & 1.4056 & 1.4186 & 1.4461 & 0.0099 \\
			\cmidrule{2-23}          & Amelia & 1.3564 & 1.3555 & 1.2798 & 1.3421 & 1.3717 & 1.4118 & 0.0224 & 1.3558 & 1.3558 & 1.3074 & 1.3474 & 1.364 & 1.4019 & 0.013 & 1.3605 & 1.3606 & 1.3331 & 1.3538 & 1.367 & 1.3887 & 0.0108 \\
			\cmidrule{2-23}          & Hmisc & 1.3535 & 1.3529 & 1.2801 & 1.3373 & 1.3708 & 1.4173 & 0.0244 & 1.355 & 1.3548 & 1.3168 & 1.3453 & 1.3643 & 1.3947 & 0.0143 & 1.3611 & 1.3608 & 1.3324 & 1.3543 & 1.3682 & 1.3951 & 0.0103 \\
			\cmidrule{2-23}          & missForest & 0.9583 & 0.9563 & 0.9172 & 0.9435 & 0.9702 & 1.046 & 0.0209 & 0.9601 & 0.9589 & 0.9373 & 0.9514 & 0.968 & 0.988 & 0.0111 & 0.9675 & 0.9672 & 0.9507 & 0.9618 & 0.971 & 1.0085 & 0.0088 \\
			\midrule
			\multirow{6}[12]{*}{\textbf{X20}} & Mean  & 0.9987 & 0.9992 & 0.9643 & 0.9904 & 1.0061 & 1.0303 & 0.0138 & 0.9994 & 0.9995 & 0.9822 & 0.9916 & 1.0055 & 1.0232 & 0.0095 & 1.0002 & 1.0006 & 0.9864 & 0.9955 & 1.0037 & 1.0224 & 0.0071 \\
			\cmidrule{2-23}          & MICE  & 0.8164 & 0.8171 & 0.7766 & 0.8071 & 0.8251 & 0.8532 & 0.0132 & 0.8398 & 0.84  & 0.8204 & 0.8344 & 0.8445 & 0.8608 & 0.008 & 0.8714 & 0.8713 & 0.8563 & 0.867 & 0.8759 & 0.8893 & 0.0062 \\
			\cmidrule{2-23}          & Mi    & 1.4108 & 1.4096 & 1.3697 & 1.4006 & 1.419 & 1.4762 & 0.0176 & 1.4113 & 1.4108 & 1.389 & 1.4061 & 1.4174 & 1.4376 & 0.0095 & 1.4153 & 1.4151 & 1.3997 & 1.4094 & 1.4211 & 1.4344 & 0.0072 \\
			\cmidrule{2-23}          & Amelia & 0.8507 & 0.8511 & 0.8153 & 0.841 & 0.8605 & 0.8812 & 0.0135 & 0.8698 & 0.8705 & 0.8459 & 0.8656 & 0.8747 & 0.8949 & 0.008 & 0.8968 & 0.8959 & 0.8789 & 0.8918 & 0.9016 & 0.9157 & 0.0067 \\
			\cmidrule{2-23}          & Hmisc & 0.819 & 0.8193 & 0.7823 & 0.8105 & 0.8279 & 0.8566 & 0.0126 & 0.8427 & 0.8428 & 0.8183 & 0.8371 & 0.8477 & 0.8637 & 0.0079 & 0.874 & 0.8739 & 0.8548 & 0.8697 & 0.8783 & 0.8954 & 0.0066 \\
			\cmidrule{2-23}          & missForest & 0.5262 & 0.5109 & 0.4911 & 0.5041 & 0.5172 & 1.0257 & 0.0867 & 0.5399 & 0.5396 & 0.5285 & 0.5357 & 0.5435 & 0.5533 & 0.0059 & 0.5734 & 0.5721 & 0.5595 & 0.5691 & 0.5743 & 0.9962 & 0.0271 \\
			\label{tbl:RMSEResultsTable}
		\end{longtable}

	\end{center}
	\newpage
	\newpage
\end{landscape}
